# Supplementary material for: Regularizing deep networks using efficient layerwise adversarial training
Source: arXiv:1705.07819 source file (2018-05-29)
Supplement: Supplementary file 1 [file appendix.tex]

\begin{center}
\section*{Appendix}
\end{center}
\subsection*{Results on Wide Residual Networks (WRN)}
Wide Residual Networks are recently proposed deep architectures that generated state of the art results on CIFAR-10 and CIFAR-100 datasets. In this experiment, we use their publicly available implementation and train them from scratch using the proposed adversarial training approach using the parameter settings described in the original paper in Section 4. Specifically, the Ours-joint approach described in Section 4.1 is used for training. As data augmentation, we applied flipping and random cropping as done in their native implementation. The results are shown in Table \ref{tab:cifar-results}. 
\begin{center}
\captionof{table}{Classification error rates (\%) on CIFAR-10 and CIFAR-100 for WideResNet (WRN) architectures. Our results are reported as average of 5 runs. For comparison we provide the published WRN baseline results. $^{(*)}$ denotes the results obtained by a single run.}
\label{tab:cifar-results}
 \begin{tabular}{| c | c | c | c |} 
 \hline
 Model & \#params & CIFAR-10 & CIFAR-100 \\ [0.5ex] 
 \hline
 WRN-28-10  & 36.5M &  4.00 & 19.25\\ 
 \hline
 WRN-28-10 with dropout  & 36.5M &  3.89 & 18.85\\ 
 \hline
 WRN-40-10 with dropout$^{*}$  & 51.0M &  3.8 & 18.3\\ 
 \hline
 WRN-28-10 with Ours-joint & 36.5M & \textbf{3.62} $\pm$ 0.05 & \textbf{17.1} $\pm$ 0.1 \\
 \hline  
\end{tabular}
\end{center}

\subsection*{Response to local perturbation depends on the Jacobian}
Let $f:\mathbb{R}^m \mapsto \mathbb{R}^n$ be a mapping between two metric spaces (euclidean, for simplicity) . Then, for $x \in \mathbb{R}^m$, let $J_f(x) \in \mathbb{R}^n \times \mathbb{R}^m$ denote the jacobian of $f$ evaluated at $x$. Let $\delta x \in \mathbb{R}^m$ be a bounded local perturbation in the neighborhood of $x$. A first order truncated expansion of $f(x+\delta x)$ is given as: 
\begin{equation*}
f(x+\delta x)=f(x)+J_f(x)^T\delta x 
\end{equation*}

We can bound the frobenius norm of the second term as follows:
\begin{align*}
& ||J_f(x)^{T}r||_F \stackrel{\text{(a)}}{\leq} ||J_f(x)||_F\;||\delta x||_2=\sqrt{\sum_{i=1}^{min(m,n)}\sigma_i^2}\;\cdot||\delta x||_2 \\
& \implies||J_f(x)^{T}\delta x||_F\leq\sqrt{\sum_{i=1}^{min(m,n)}\sigma_i^2}\;\cdot||\delta x||_2
\end{align*}
where $||\cdot||_F$ denotes the frobenius norm; for vectors, it is the same as the $L_2$ norm and $\sigma_i$ denotes the $i^{th}$ singular value of the Jacobian; (a) is a direct application of Cauchy-Schwarz inequality. Applying this result to the singular value spectra plotted in Figure 2 in the paper, we see that the base network without adversarial training is extremely sensitive to local perturbations compared to adversarially trained networks using FGS and the proposed approach. 

\subsection*{Setting $\epsilon$ parameter}
Following the notation from Section 3, let $\nabla_{l}\mathcal{J}(\theta,x,y)$ denote the gradient of the loss function backpropagated to the $l^{th}$ layer. Let $M = max(\nabla_{l}\mathcal{J}(\theta,x,y))$, $m = min(\nabla_{l}\mathcal{J}(\theta,x,y))$. Then, the value of $\epsilon$ for each layer is calculated as: ${\epsilon}_{l}=\epsilon\;\cdot(M-m)\; \forall l$, where $\epsilon\in\{10,20,30\}$. The exact value is cross-validated using a held out set. In practice, we found our training approach to not be overly sensitive to $\epsilon$. We tuned $\epsilon$ only for the VGG network on CIFAR-10 and used the same value for all the other networks such as ResNets and WideResNets on both CIFAR-10 and CIFAR-100 datasets. Note that, for cases where a fixed value of $\epsilon$ is specified such as in Figure 1 in the paper, the same value is used for all layers ignoring the normalizing factor, $(M-m)$.
